# Supplementary material for: Single-Modal Entropy based Active Learning for Visual Question Answering
Source: arXiv:2110.10906 source file (2021-11-18)
Supplement: Supplementary file 2 [file Supplementary_AAAI.tex]

\relax
%File: formatting-instructions-latex-2021.tex
%release 2021.1
\documentclass[letterpaper]{article} % DO NOT CHANGE THIS
\usepackage{aaai21}  % DO NOT CHANGE THIS
\usepackage{times}  % DO NOT CHANGE THIS
\usepackage{helvet} % DO NOT CHANGE THIS
\usepackage{courier}  % DO NOT CHANGE THIS
\usepackage[hyphens]{url}  % DO NOT CHANGE THIS
\usepackage{graphicx} % DO NOT CHANGE THIS
\urlstyle{rm} % DO NOT CHANGE THIS
  % DO NOT CHANGE THIS
\usepackage{natbib}  % DO NOT CHANGE THIS AND DO NOT ADD ANY OPTIONS TO IT
\usepackage{caption} % DO NOT CHANGE THIS AND DO NOT ADD ANY OPTIONS TO IT
\frenchspacing  % DO NOT CHANGE THIS
\setlength{\pdfpagewidth}{8.5in}  % DO NOT CHANGE THIS
\setlength{\pdfpageheight}{11in}  % DO NOT CHANGE THIS

\usepackage[utf8]{inputenc} % allow utf-8 input
\usepackage[T1]{fontenc}    % use 8-bit T1 fonts
\usepackage{booktabs}       % professional-quality tables
\usepackage{amsfonts}       % blackboard math symbols
\usepackage{nicefrac}       % compact symbols for 1/2, etc.
\usepackage{microtype}      % microtypography

\usepackage[ruled,vlined]{algorithm2e}
\usepackage{wrapfig}
\usepackage{mathtools}
\usepackage{color}
\usepackage{paralist}
\usepackage{subfigure}
\usepackage{multirow}
\usepackage[normalem]{ulem} % for sout
%\nocopyright
%PDF Info Is REQUIRED.
% For /Author, add all authors within the parentheses, separated by commas. No accents or commands.
% For /Title, add Title in Mixed Case. No accents or commands. Retain the parentheses.
\pdfinfo{
/Title (AAAI Press Formatting Instructions for Authors Using LaTeX -- A Guide)
/Author (AAAI Press Staff, Pater Patel Schneider, Sunil Issar, J. Scott Penberthy, George Ferguson, Hans Guesgen, Francisco Cruz, Marc Pujol-Gonzalez)
/TemplateVersion (2021.1)
} %Leave this
% /Title ()
% Put your actual complete title (no codes, scripts, shortcuts, or LaTeX commands) within the parentheses in mixed case
% Leave the space between \Title and the beginning parenthesis alone
% /Author ()
% Put your actual complete list of authors (no codes, scripts, shortcuts, or LaTeX commands) within the parentheses in mixed case.
% Each author should be only by a comma. If the name contains accents, remove them. If there are any LaTeX commands,
% remove them.

%\DeclareRobustCommand\onedot{\futurelet\@let@token\@onedot}
\def\@onedot{\ifx\@let@token.\else.\null\fi\xspace}

\newcommand{\Cref}[1]{Chap.~\ref{#1}}

\setcounter{secnumdepth}{0} %May be changed to 1 or 2 if section numbers are desired.

% The file aaai21.sty is the style file for AAAI Press
% proceedings, working notes, and technical reports.
%

% Title

% Your title must be in mixed case, not sentence case.
% That means all verbs (including short verbs like be, is, using,and go),
% nouns, adverbs, adjectives should be capitalized, including both words in hyphenated terms, while
% articles, conjunctions, and prepositions are lower case unless they
% directly follow a colon or long dash

\title{---Supplementary Material---\\Single-Modal Entropy based Active Learning for Visual Question Answering}

\author{

    %Authors
    % All authors must be in the same font size and format.
    Written by AAAI Press Staff\\%\textsuperscript{\rm 1}\thanks{With help from the AAAI Publications Committee.}\\
    %AAAI Style Contributions by Pater Patel Schneider,
    %Sunil Issar,  \\
    %J. Scott Penberthy,
    %George Ferguson,
    %Hans Guesgen,
    %Francisco Cruz,
    %Marc Pujol-Gonzalez
    %\\
}
\affiliations{
    %Afiliations

    \textsuperscript{\rm 1}Association for the Advancement of Artificial Intelligence\\
    %If you have multiple authors and multiple affiliations
    % use superscripts in text and roman font to identify them.
    %For example,

    % Sunil Issar, \textsuperscript{\rm 2}
    % J. Scott Penberthy, \textsuperscript{\rm 3}
    % George Ferguson,\textsuperscript{\rm 4}
    % Hans Guesgen, \textsuperscript{\rm 5}.
    % Note that the comma should be placed BEFORE the superscript for optimum readability

    2275 East Bayshore Road, Suite 160\\
    Palo Alto, California 94303\\
    % email address must be in roman text type, not monospace or sans serif
    %publications21@aaai.org

    % See more examples next
}
\iffalse
%Example, Single Author, ->> remove \iffalse,\fi and place them surrounding AAAI title to use it
\title{My Publication Title --- Single Author}
\author {
    % Author
    Author Name \\
}

\affiliations{
    Affiliation \\
    Affiliation Line 2 \\
    name@example.com
}
\fi

\iffalse
%Example, Multiple Authors, ->> remove \iffalse,\fi and place them surrounding AAAI title to use it
\title{My Publication Title --- Multiple Authors}
\author {
    % Authors

        First Author Name,\textsuperscript{\rm 1}
        Second Author Name, \textsuperscript{\rm 2}
        Third Author Name \textsuperscript{\rm 1} \\
}
\affiliations {
    % Affiliations
    \textsuperscript{\rm 1} Affiliation 1 \\
    \textsuperscript{\rm 2} Affiliation 2 \\
    firstAuthor@affiliation1.com, secondAuthor@affilation2.com, thirdAuthor@affiliation1.com
}
\fi
\begin{document}

\maketitle

\input{5_sec_supplementary}

%\clearpage
%\section*{References}
{\small
\bibliography{egbib}
}

\end{document}
